# Supplementary material for: A new symmetry-based framework for discovering minimum energy pathways
Source: arXiv:1804.06798 ancillary file (2018-04-18)
Supplement: Supplementary file 1 [file supplementary.pdf]

# SUPPLEMENTARY MATERIAL

## Supplementary Note 1: Determining the distortion symmetry group of a path.

More formally, the distortion symmetry group of any path can be found as follows: We first find the intersection group ( $H$ ) of the conventional spatial symmetry operations of all the images in a path. Then we identify possible “starred” operations ( $A^*$ ) that map the structure at the reaction coordinate  $\lambda$  to the ones at  $-\lambda$ . We can write these operations as  $A^* = A1^*$ , where  $A$  would be a symmetry operation of the structure at  $\lambda = 0$ , and  $1^*$  is an antisymmetry operation that acts as follows:  $1^*(\lambda) = -\lambda$ . The distortion group can then be written as  $H \cup A^*H$ . In the case of the initial path in **Figure 1**,  $H = \{1, m_y\}$  and  $A^* = \{m_x^*, 2_z^*\}$ , resulting in a distortion group of  $m_x^* m_y 2_z^*$ . If no  $A^*$  operations exist, then the distortion symmetry group of the path will be  $H$ .

|            | <b>1</b> | <b><math>m_x^*</math></b> | <b><math>m_y</math></b> | <b><math>2_z^*</math></b> | <b>Kernel</b>                       |
|------------|----------|---------------------------|-------------------------|---------------------------|-------------------------------------|
| $\Gamma_1$ | 1        | 1                         | 1                       | 1                         | <b><math>m_x^* m_y 2_z^*</math></b> |
| $\Gamma_2$ | 1        | 1                         | -1                      | -1                        | <b><math>m_x^*</math></b>           |
| $\Gamma_3$ | 1        | -1                        | 1                       | -1                        | <b><math>m_y</math></b>             |
| $\Gamma_4$ | 1        | -1                        | -1                      | 1                         | <b><math>2_z^*</math></b>           |

**Supplementary Table 1.** The character table of the distortion group  $m_x^* m_y 2_z^*$ . The distortion group resulting from the kernel of each irrep is shown in the last column.

|          | <b>1</b> | <b><math>2_1</math></b> | <b><math>2_y^*</math></b> | <b><math>2_x^*</math></b> | <b><math>\bar{1}^*</math></b> | <b><math>m_z^*</math></b> | <b>c</b> | <b><math>m_x</math></b> | <b>Kernel</b>               |
|----------|----------|-------------------------|---------------------------|---------------------------|-------------------------------|---------------------------|----------|-------------------------|-----------------------------|
| $Y_{1+}$ | 1        | 1                       | 1                         | 1                         | 1                             | 1                         | 1        | 1                       | <b><math>Pm^* ma</math></b> |
| $Y_{2+}$ | 1        | 1                       | -1                        | -1                        | 1                             | 1                         | -1       | -1                      | <b><math>Pnm^* a</math></b> |
| $Y_{3+}$ | 1        | -1                      | 1                         | -1                        | 1                             | -1                        | 1        | -1                      | <b><math>Pbcn^*</math></b>  |
| $Y_{4+}$ | 1        | -1                      | -1                        | 1                         | 1                             | -1                        | -1       | 1                       | <b><math>Pnn^* m</math></b> |
| $Y_{1-}$ | 1        | 1                       | 1                         | 1                         | -1                            | -1                        | -1       | -1                      | <b><math>Pnn^* a</math></b> |
| $Y_{2-}$ | 1        | 1                       | -1                        | -1                        | -1                            | -1                        | 1        | 1                       | <b><math>Pn^* ma</math></b> |
| $Y_{3-}$ | 1        | -1                      | 1                         | -1                        | -1                            | 1                         | -1       | 1                       | <b><math>Pm^* mn</math></b> |
| $Y_{4-}$ | 1        | -1                      | -1                        | 1                         | -1                            | 1                         | 1        | -1                      | <b><math>Pbcm^*</math></b>  |

**Supplementary Table 2.** The character table of the distortion group  $Cmcm^*$  at the high symmetry  $Y$   $k$ -point  $k = (1, 0, 0)$ . The distortion group resulting from the kernel of each irrep is also shown.

|               | <b>1</b> | <b>3</b> | <b><math>2^*</math></b> | <b><math>\bar{1}^*</math></b> | <b><math>\bar{3}^*</math></b> | <b>c</b> | <b>Kernel</b>                    |
|---------------|----------|----------|-------------------------|-------------------------------|-------------------------------|----------|----------------------------------|
| $\Gamma_{1+}$ | 1        | 1        | 1                       | 1                             | 1                             | 1        | <b><math>R\bar{3}^* c</math></b> |
| $\Gamma_{2+}$ | 1        | 1        | -1                      | 1                             | 1                             | -1       | <b><math>R\bar{3}^*</math></b>   |
| $\Gamma_{3+}$ | 2        | -1       | 0                       | 2                             | -1                            | 0        | <b><math>P\bar{1}^*</math></b>   |
| $\Gamma_{1-}$ | 1        | 1        | 1                       | -1                            | -1                            | -1       | <b><math>R32^*</math></b>        |
| $\Gamma_{2-}$ | 1        | 1        | -1                      | -1                            | -1                            | 1        | <b><math>R3c</math></b>          |
| $\Gamma_{3-}$ | 2        | -1       | 0                       | -2                            | 1                             | 0        | <b><math>P1</math></b>           |

**Supplementary Table 3.** The character table of the distortion group  $R\bar{3}^* c$  at  $\Gamma$  point  $k = (0, 0, 0)$ . The distortion group resulting from the kernel of each irrep is also shown.

|               | <b>1</b> | <b>2<sub>1</sub></b> | <b>2<sub>y</sub><sup>*</sup></b> | <b>2<sub>x</sub><sup>*</sup></b> | <b><math>\bar{1}^*</math></b> | <b><math>m_z^*</math></b> | <b>c</b> | <b><math>m_x</math></b> | <b>Kernel</b>                  |
|---------------|----------|----------------------|----------------------------------|----------------------------------|-------------------------------|---------------------------|----------|-------------------------|--------------------------------|
| $\Gamma_{1+}$ | 1        | 1                    | 1                                | 1                                | 1                             | 1                         | 1        | 1                       | <b><math>Pm^*ma</math></b>     |
| $\Gamma_{2+}$ | 1        | -1                   | -1                               | 1                                | 1                             | -1                        | -1       | 1                       | <b><math>P2^*/a</math></b>     |
| $\Gamma_{3+}$ | 1        | 1                    | -1                               | -1                               | 1                             | 1                         | -1       | -1                      | <b><math>P2_1/m^*</math></b>   |
| $\Gamma_{4+}$ | 1        | -1                   | 1                                | -1                               | 1                             | -1                        | 1        | -1                      | <b><math>P2^*/m</math></b>     |
| $\Gamma_{1-}$ | 1        | 1                    | 1                                | 1                                | -1                            | -1                        | -1       | -1                      | <b><math>P2_12^*2^*</math></b> |
| $\Gamma_{2-}$ | 1        | -1                   | -1                               | 1                                | -1                            | 1                         | 1        | -1                      | <b><math>Pm^*m2^*</math></b>   |
| $\Gamma_{3-}$ | 1        | 1                    | -1                               | -1                               | -1                            | -1                        | 1        | 1                       | <b><math>P2_1ma</math></b>     |
| $\Gamma_{4-}$ | 1        | -1                   | 1                                | -1                               | -1                            | 1                         | -1       | 1                       | <b><math>Pm^*2^*a</math></b>   |

**Supplementary Table 4.** The character table of the distortion group  $Pm^*ma$  at  $\Gamma$  point  $k = (0, 0, 0)$ . The distortion group resulting from the kernel of each irrep is also shown.

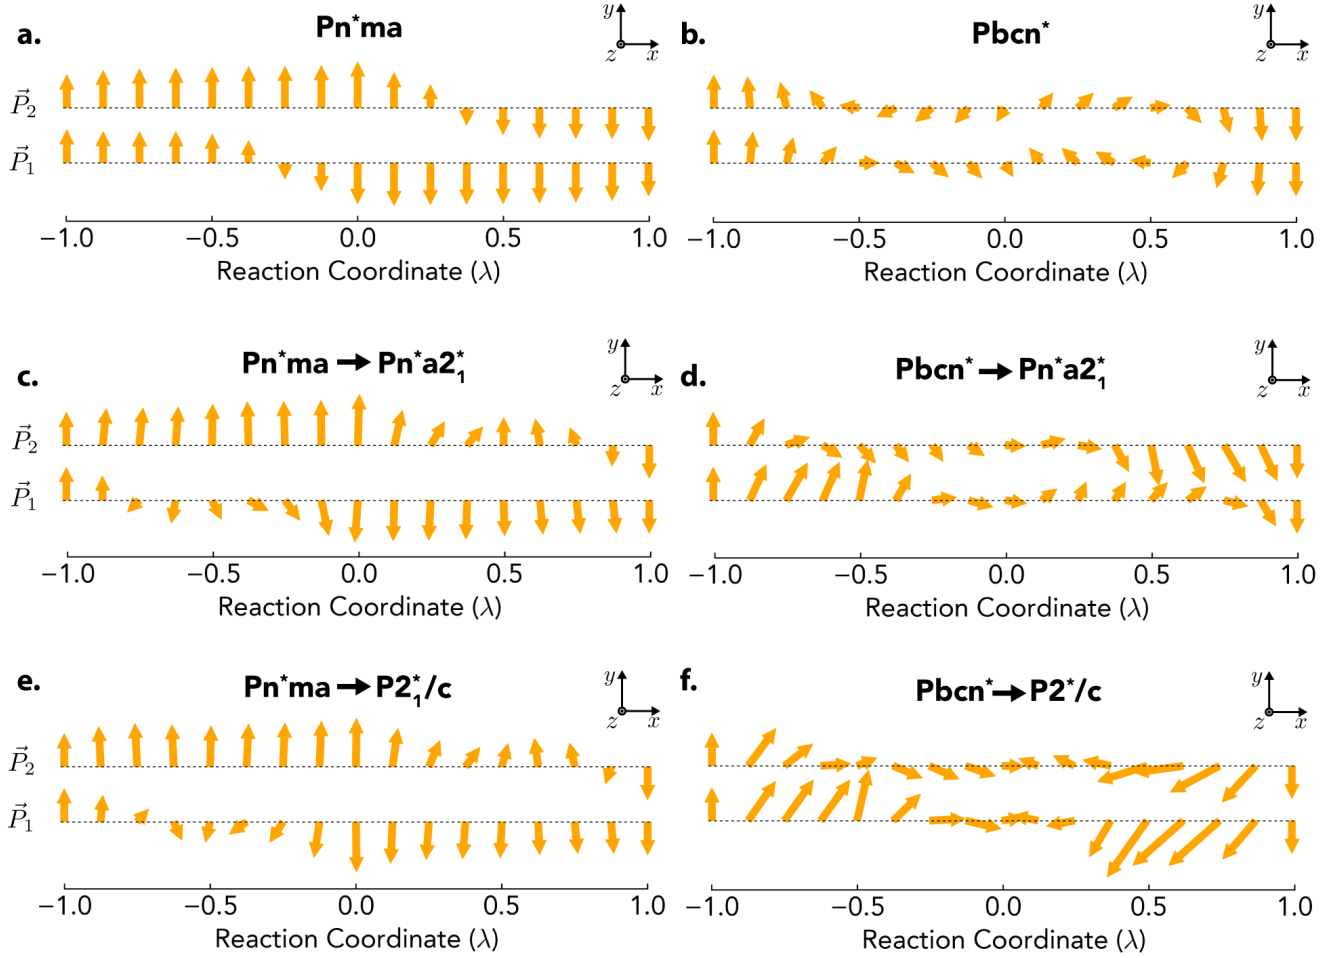

**Supplementary Figure 1.** Arrows indicating the direction of the polarization in each slab of the  $Ca_3Ti_2O_7$  cell as a function of reaction coordinate. Data is shown for the two-step paths with  $Pn^*ma$  and  $Pbcn^*$  symmetry, as well as for the low energy four step paths resulting from their perturbation.

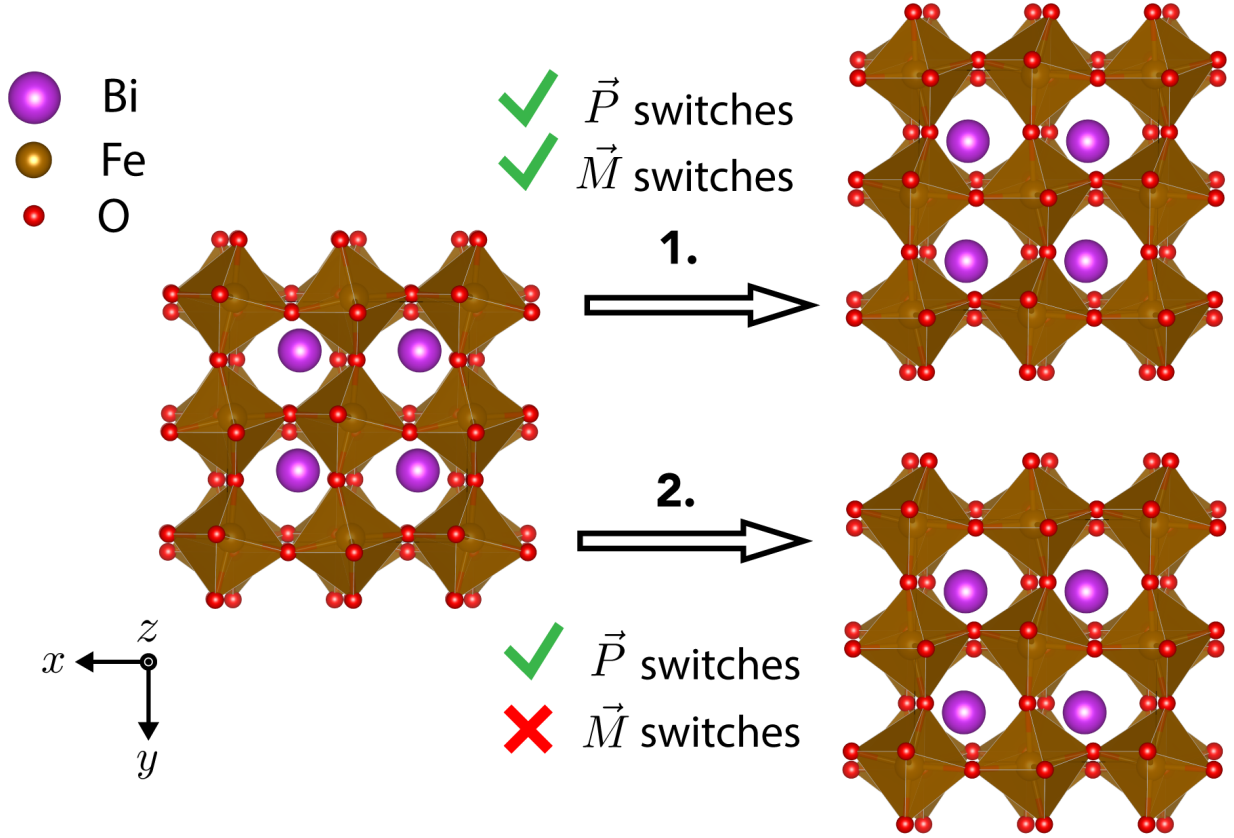

**Supplementary Figure 2.** The pseudocubic ( $Z = 8$ ) supercells of the initial (left) and final states (right) of the  $\text{BiFeO}_3$  switching pathways. The path with the rotation of the oxygen octahedra is labelled as **1**, with the other that does not include them labeled as **2**. Both resulting paths involve the reversal of the polarization ( $\vec{P}$ ), while reversal of the oxygen octahedra necessitates a switching of the magnetization ( $\vec{M}$ ) for path **1**.

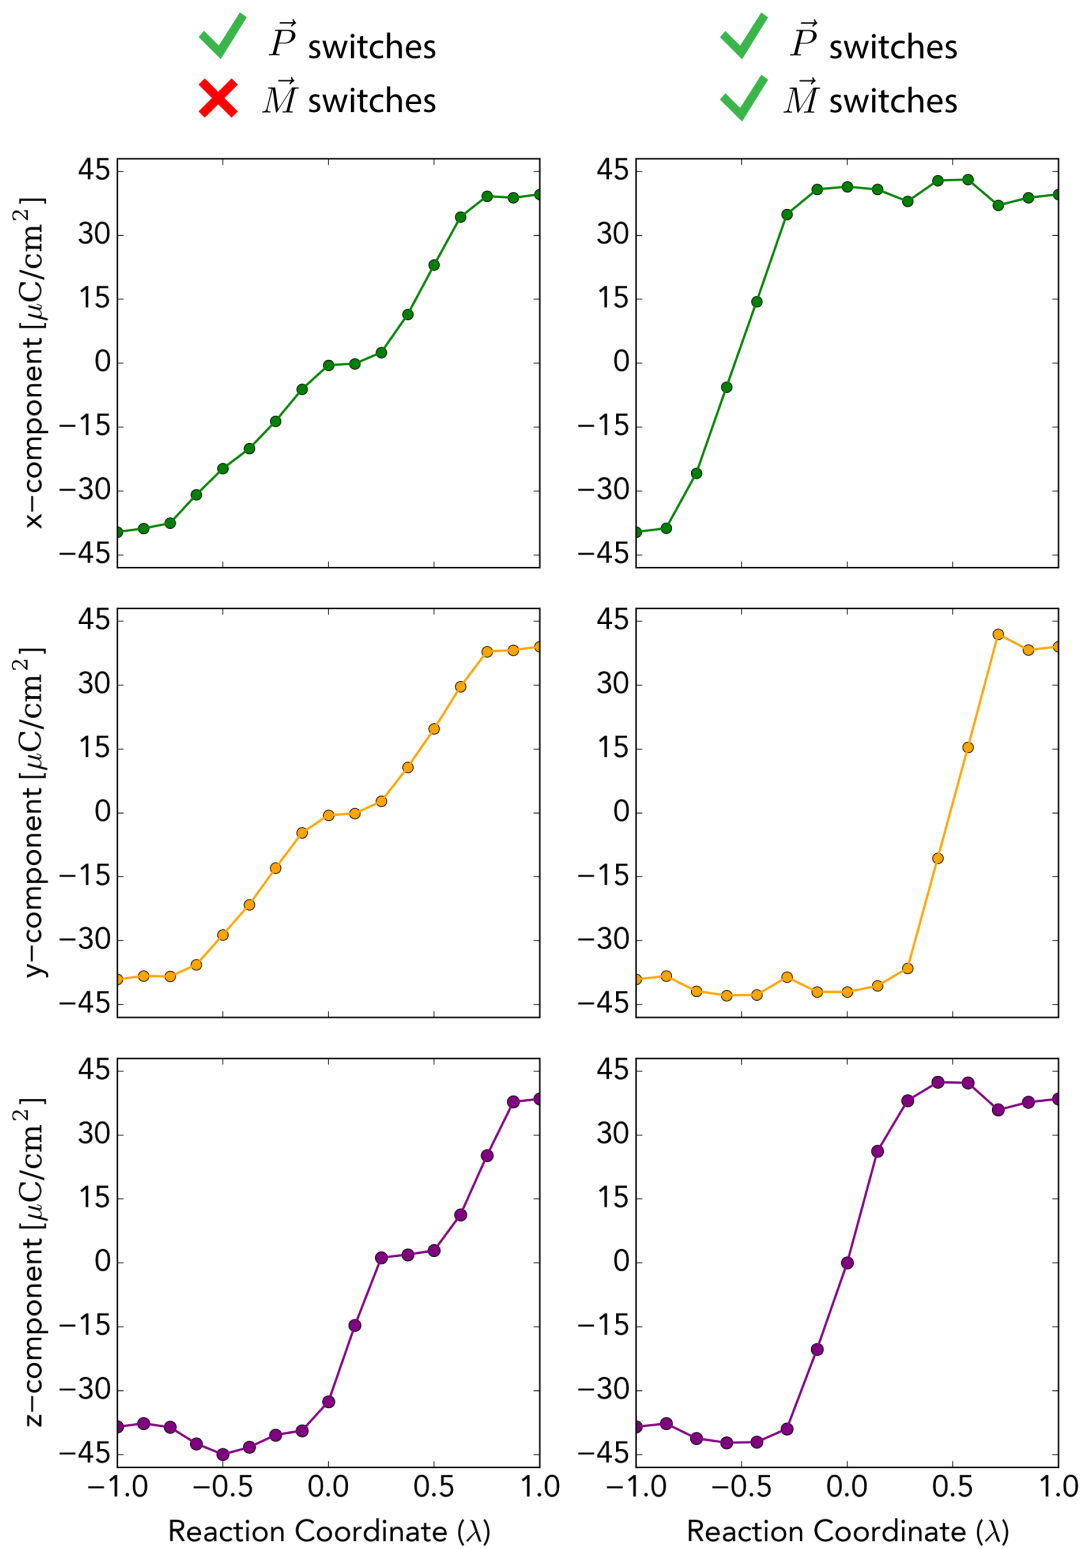

**Supplementary Figure 3.** Polarization data as a function of reaction coordinate for both  $\text{BiFeO}_3$  switching pathways calculated using ionic charges.

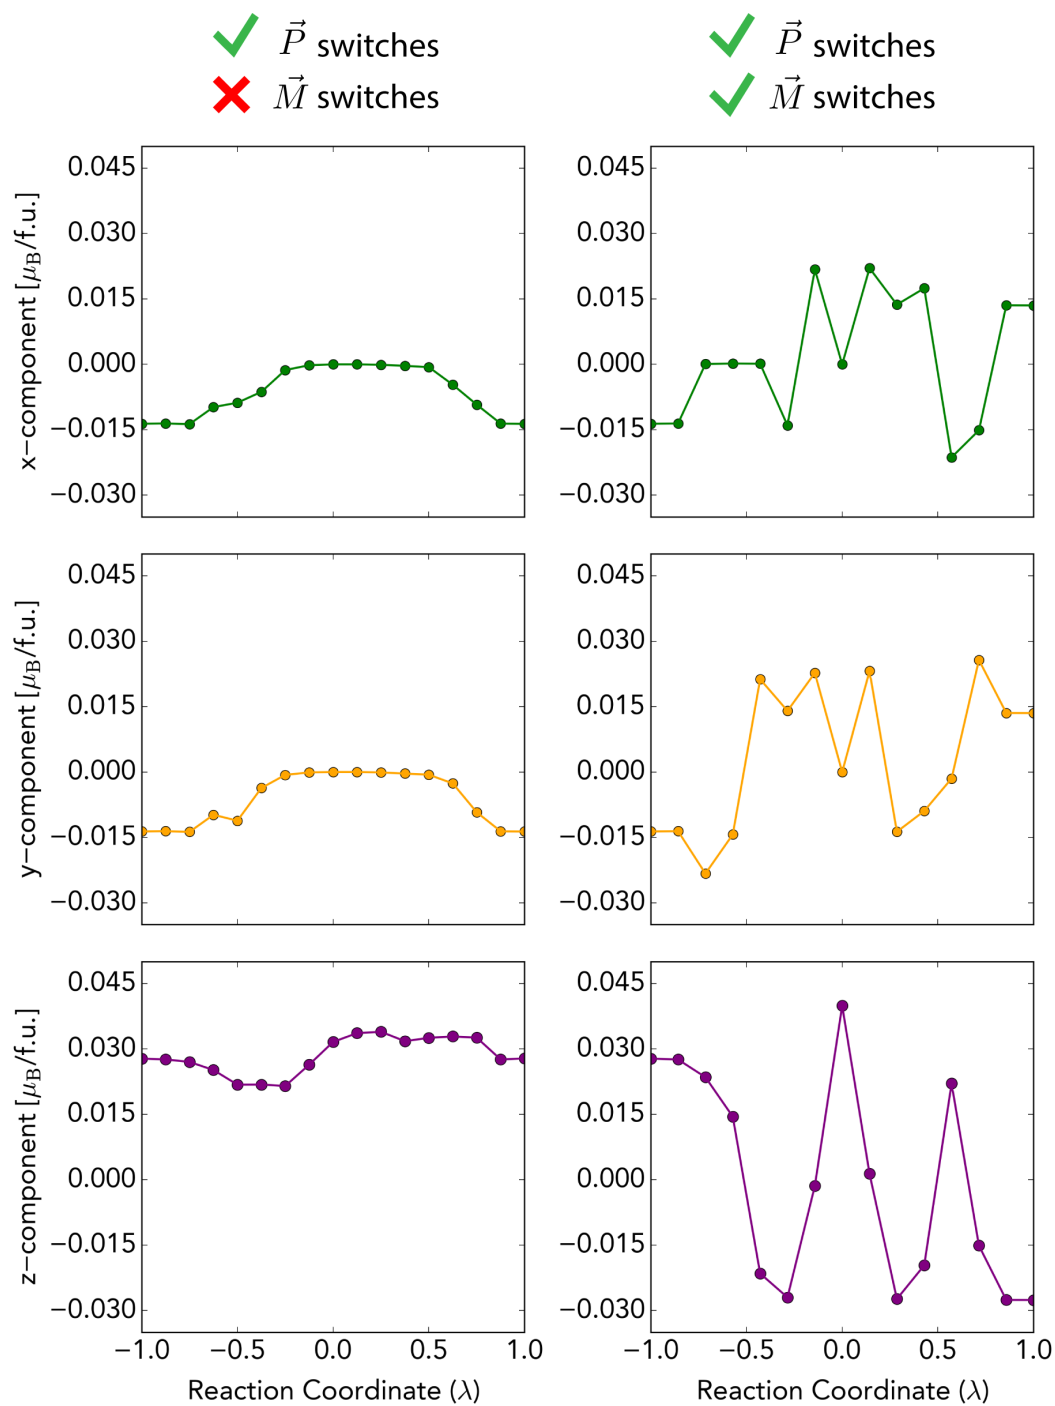

**Supplementary Figure 4.** Magnetization data as a function of reaction coordinate for both  $\text{BiFeO}_3$  switching pathways.

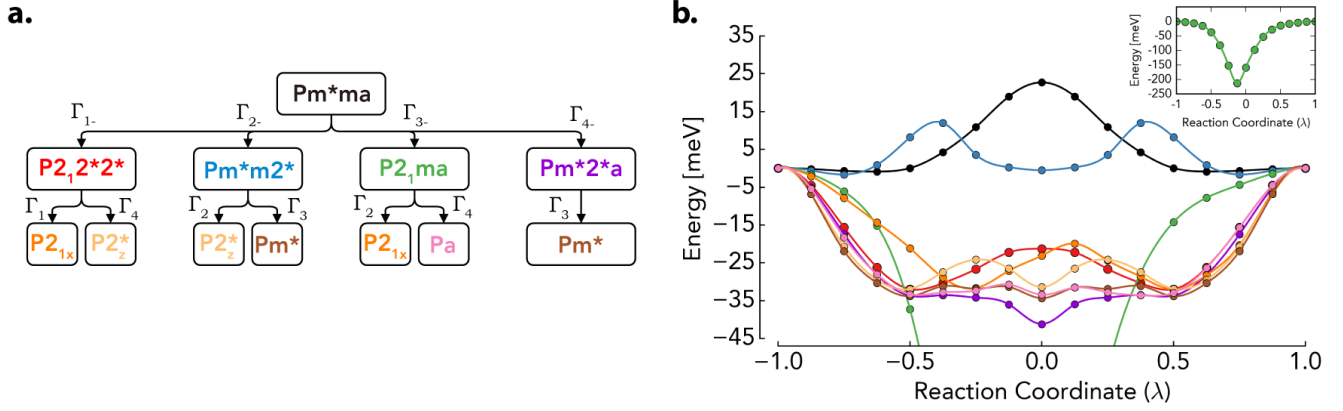

**Supplementary Figure 5.** (a) Tree of perturbations showing the resulting distortion group of the paths presented in panel **b**. (b) Energy relative to the initial and final states shown in **Figure 3a** as a function of reaction coordinate for NEB calculations involving changing lattice vectors via the generalized solid-state (G-SSNEB) algorithm. The images of lowest energy in the  $Pm2^*a$  and  $P2_1ma$  paths correspond to all unit cells in the supercell structure taking on the form of the ferroelectric orthorhombic and tetragonal ground states of  $PbTiO_3$ . The full energy profile for the  $P2_1ma$  path is shown in the inset plot.

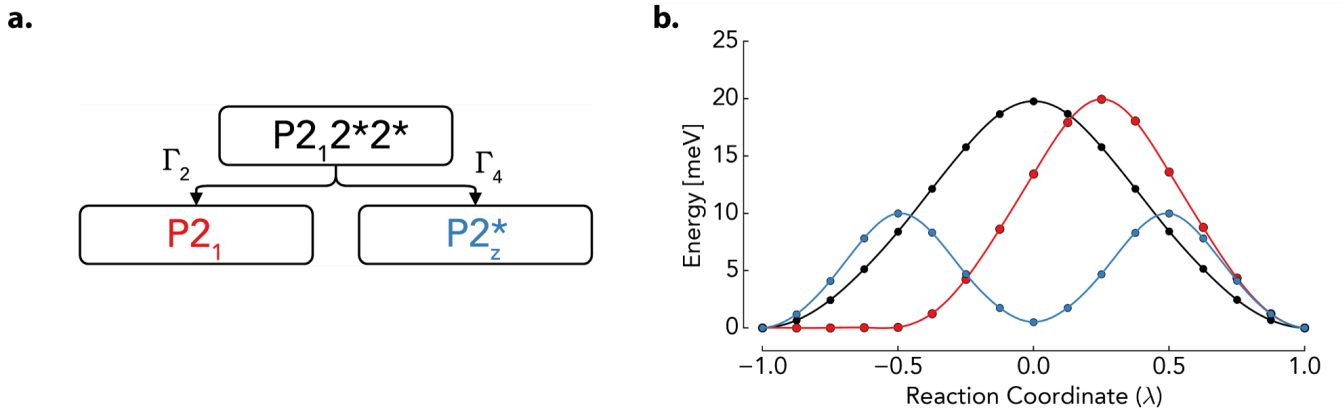

**Supplementary Figure 6.** (a) Tree of perturbations showing the resulting distortion group of the paths presented in panel **b**. (b) Energy relative to the initial and final states from NEB calculations employing the generalized solid-state (G-SSNEB) algorithm. These initial and final states for these calculations were constructed from the ground state structures found at  $\lambda = 0.5$  in **Supplementary Figure 5b**. The  $P2_12^*2^*$ ,  $P2_1$  and  $P2_z^*$  paths are equivalent to the paths in **Supplementary Figure 5b** with the same path symmetry.

## Supplementary Note 2: Implementation outline of the distortion symmetry tool into the commercial NEB codes.

In order to complete this work, the ability to automatically detect the distortion symmetry of a path and generate symmetry-adapted perturbations was implemented into a standalone piece of Python code, as well as the open source Quantum-ESPRESSO [1] software package. These use the open source package SPGLIB [2] to obtain the symmetry of the static structures that make up the path, from which the path symmetry group is generated. In order to obtain symmetry-adapted path perturbations, the matrix representation of all distortion group elements for every irrep are required. Since distortion groups are isomorphic to space groups, the listing of all irrep matrices of the space groups by Stokes et al. [3] is used. The chart in **Supplementary Figure 4** illustrates the steps that both implementations take, as well as how they interface with the rest of the NEB algorithm. The steps highlighted in blue are ones that both implementations take to pre-process path data. The ones in green illustrate a potential speed up (**Supplementary Figure 8**) that is enabled specifically in the Quantum-ESPRESSO implementation if any “starred” elements exist in the distortion group of the initial path. By having this kind of element, it is known *a priori* that the paths energy profile will be symmetric about  $\lambda = 0$ . This allows the NEB algorithm to only require forces and energies for half of the images along the path. Both of these implementations are continuing to be developed, and will be released to the public as part of a separate publication.

- 
- [1] P. Giannozzi, S. Baroni, N. Bonini, M. Calandra, R. Car, C. Cavazzoni, D. Ceresoli, G. L. Chiarotti, M. Cococcioni, I. Dabo, A. Dal Corso, S. de Gironcoli, S. Fabris, G. Fratesi, R. Gebauer, U. Gerstmann, C. Gougoussis, A. Kokalj, M. Lazzeri, L. Martin-Samos, N. Marzari, F. Mauri, R. Mazzarello, S. Paolini, A. Pasquarello, L. Paulatto, C. Sbraccia, S. Scandolo, G. Sclauzero, A. P. Seitsonen, A. Smogunov, P. Umari, and R. M. Wentzcovitch, *Journal of Physics: Condensed Matter* **21**, 395502 (2009).
  - [2] A. Togo, “Spglib,” (2009).
  - [3] H. T. Stokes, B. J. Campbell, and R. Cordes, *Acta Crystallographica Section A Foundations of Crystallography* **69**, 388 (2013).

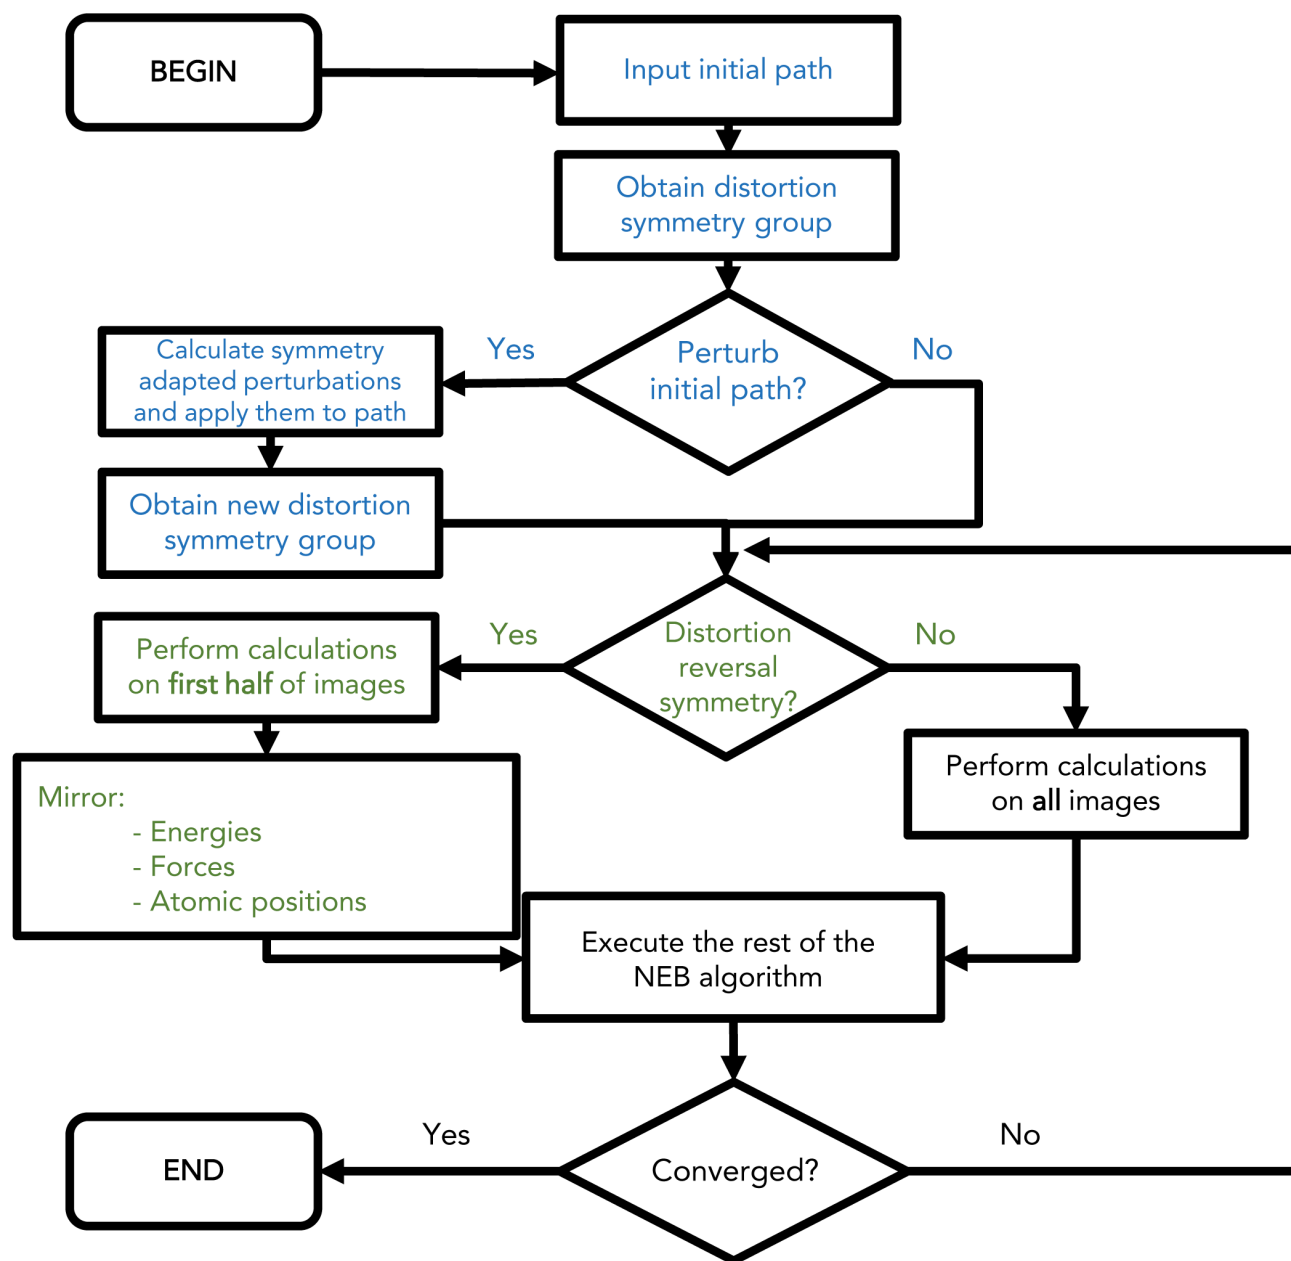

**Supplementary Figure 7.** A flowchart showing the complete symmetry-adapted NEB algorithm. The blue highlighted steps are ones that both the Python and Quantum-ESPRESSO [1] implementations take to pre-process path data and generate new initial paths from symmetry-adapted perturbations. The green steps illustrate the potential calculation speed-up that exists in the latter by considering if any “starred” elements exist in the distortion group of the initial path.

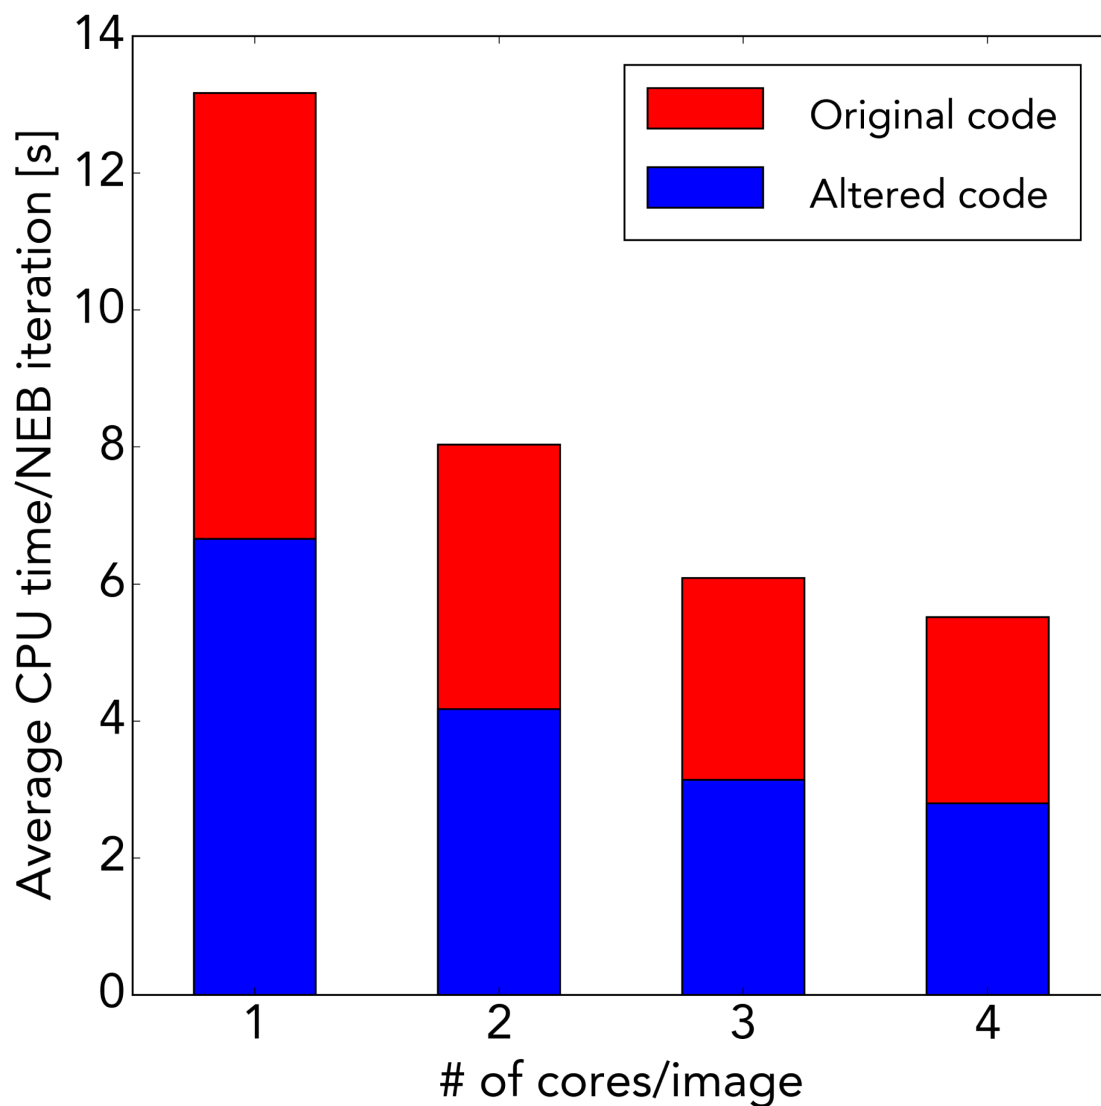

**Supplementary Figure 8.** A flowchart illustrating the calculation speed-up possible for paths with “starred” symmetry operations in their distortion symmetry group. For the same number of cores per image, a two-fold speed up is observed by only requiring energy and force calculations for half of the images in the path. The data shown is for a bulk  $180^\circ$  polarization switching pathway in  $\text{PbTiO}_3$  using code implemented in the Quantum-ESPRESSO [1] package.
